# Supplementary material for: Quantum-Like Contextuality in Large Language Models
Source: arXiv:2412.16806 source file (2024-12-21)
Supplement: Supplementary file 1 [file appendix.tex]

\section{Special models}
\subsection{PR boxes}
A PR box is a special model that maximises the degree of contextuality, that is, maximally contextual. 
The defining feature of a PR box is that the joint distribution of any context is either perfectly correlated or perfectly anti-correlated.
If the number of anti-correlated contexts is odd, then the model is a PR box.

An example of a PR box is the following:
\begin{table}[h]
  \centering
  \begin{tabular}{r|ccccc}
  & $(0, 0)$ & $(0, 1)$ & $(1, 0)$ & $(1, 1)$  \\ \hline
  $(x_1, x_2)$ & $1 / 2$ & $0$ & $0$ & $1 / 2$ \\
  $(x_2, x_3)$ & $1 / 2$ & $0$ & $0$ & $1 / 2$ \\
  $(x_3, x_4)$ & $1 / 2$ & $0$ & $0$ & $1 / 2$ \\
  $(x_4, x_1)$ & $0$ & $1 / 2$ & $1 / 2$ & $0$ \\
  \end{tabular}
\end{table}

The contextual fraction of a PR box is $1$.
\subsection{PR-like models}
A PR-like model is one that shares the same possibility reduction as a PR box.
A family of PR-like models can be parametrised by a one real parameter $\epsilon_i$ for each context $i$.
\begin{table}[h]
  \centering
  \begin{tabular}{r|ccccc}
  & $(0, 0)$ & $(0, 1)$ & $(1, 0)$ & $(1, 1)$  \\ \hline
  $(x_1, x_2)$ & $(1+\epsilon_{1,2})/2$ & $0$ & $0$ & $(1-\epsilon_{1,2})/2$ \\
  $(x_2, x_3)$ & $(1+\epsilon_{2,3})/2$ & $0$ & $0$ & $(1-\epsilon_{2,3})/2$ \\
  $(x_3, x_4)$ & $(1+\epsilon_{3,4})/2$ & $0$ & $0$ & $(1-\epsilon_{3,4})/2$ \\
  $(x_4, x_1)$ & $0$ & $(1+\epsilon_{4,1})/2$ & $(1-\epsilon_{4,1})/2$ & $0$
  \end{tabular}
\end{table}
Note that the PR box is a special case of the PR-like model, where $\epsilon_i = 0$ for all $i$.
Thus the paramters $\epsilon_{i, i \oplus 1}$ can be seen as the deviation from the PR box.
The contextual fraction of a PR-like model is 1. 
The signalling fraction is given by the maximum of the absolute values of the parameters $\epsilon_{i, i \oplus 1}$.
\begin{align}
    \text{SF}\left(\{\epsilon_{i, i \oplus 1}\}\right) = \max_i |\epsilon_{i, i \oplus 1}|.
\end{align}
The formula for Direct influence is given by
\begin{align}
   \Delta(\{\epsilon_{i, i \oplus 1}\}) = |\epsilon_{1, 2} - \epsilon_{2, 3}| + |\epsilon_{2, 3} - \epsilon_{3, 4}| + \cdots + |\epsilon_{n, 1} + \epsilon_{1, 2}|.
\end{align}

\subsection{symmetric models}
The symmetric models are those that are invariant under permutations of the outcome labels.
To be precise, the joint distribution of any context is invariant under permutations of the outcome labels.

\begin{Theorem}
    All symmetric models are non-signalling. 
\end{Theorem}
\begin{proof}
    The proof is trivial once it is realised that every marginal distribution is a uniform one, and thus independent of the context.
    Consider the joint distribution of a context $(x, y)$.
    The fact that the model is symmetric means that
    \begin{align}
        p(x=0, y=0) = p(x=1, y=1)
    \end{align},
    and
    \begin{align}
        p(x=0, y=1) = p(x=1, y=0).
    \end{align}
    
    To prove that all marginal distributions are uniform, consider the marginal distribution of $x$:
    \begin{align}
      p(x=0) = \sum_{o_y \in \{0, 1\}} p(x=0, y=o_y)
  \end{align},
  Using the fact that the model is symmetric, we have
  \begin{align}
      p(x=0) &= \sum_{o_y \in \{1, 0\}} p(x=1, y=o_y) \\
      &= p(x=1).
  \end{align}
\end{proof}

The above theorem can be generalised to symmetric models with arbitrary number of outcomes per observable. We formalise the notion of symmetry as the group action of a permutation group on the set of outcomes.
If the group action is transitive, meaning that for any pair of outcomes $o_1$ and $o_2$, there exists a permutation $g$ such that $g(o_1) = o_2$, then we can prove that every marginal distribution is uniform using the same argument as above.

\begin{Theorem}
  For all symmetric models of the Bell-CHSH scenario, the inequality that saturates the normalised violation bound determined by contextual fraction is the canonical Bell-CHSH inequality. (The reverse is also true. Maybe.)
\end{Theorem}

\begin{proof}
    Consider the dual program of the linear program that determines the CF. See Abramsky 2017. 
    
\end{proof}
\section{BERT}
The core of BERT (Bidirectional Encoder Representations from Transformers) is a neural model that convert a sequence of tokens into a sequence of (contextualised) vectors.
It does so by first converting each token into its embedding vector, and then passing the sequence of embedding vectors through a stack of transformer layers.
The results of the transformer layers are considered the contextualised output vectors of the input tokens.
One usage of BERT is to predict a masked token in a sequence of tokens.
For example, given the sequence of tokens ``I want to \texttt{[MASK]} a car'', BERT would predict the masked token to be ``buy''.
This is done by training a so called ``masked language model'' prediction head, which takes the contextualised output vector corresponding to the masked token as input, and outputs a logit for each token in the vocabulary. The logits are then converted into probabilities using a softmax function.
In this prediction head, the contextualised output vector of the masked token is fed into a feedforward layer, with an nonlinear activation function in between.  
The logits are then computed by multiplying (dot product) the output from the feedforward layer with the embedding of the token, followed by a scalar bias term.
To be precise, the logit for the $i-th$ token in the vocabulary is computed as follows:
\begin{align}
    l_i = \mathbf{p} \cdot \mathbf{x}_i + b_i
\end{align}
where $\mathbf{p}$ is the contextualised output vector of the masked token, $\mathbf{x}_i$ is the embedding vector of the $i-th$ token in the vocabulary, and $b_i$ is the bias term for the $i-th$ token in the vocabulary.
The probability of the $i-th$ token in the vocabulary is then computed as follows:
\begin{align}
    p_i = \frac{\exp(l_i)}{\sum_{j=1}^{|V|} \exp(l_j)}    
\end{align}

The prediction head of the BERT model we have the following architecture:
% make the listing smaller by using \footnotesize
{
\footnotesize
\begin{lstlisting}
    BertLMPredictionHead(
  (transform): BertPredictionHeadTransform(
    (dense): Linear(in_features=768, out_features=768, bias=True)
    (transform_act_fn): GELUActivation()
    (LayerNorm): LayerNorm((768,), eps=1e-12, elementwise_affine=True)
  )
  (decoder): Linear(in_features=768, out_features=30522, bias=True)
)
\end{lstlisting}
}

The encoder of the BERT model we have the following architecture:
{
\footnotesize
\begin{lstlisting}
 BertModel(
  (embeddings): BertEmbeddings(
    (word_embeddings): Embedding(30522, 768, padding_idx=0)
    (position_embeddings): Embedding(512, 768)
    (token_type_embeddings): Embedding(2, 768)
    (LayerNorm): LayerNorm((768,), eps=1e-12, elementwise_affine=True)
    (dropout): Dropout(p=0.1, inplace=False)
  )
  (encoder): BertEncoder(
    (layer): ModuleList(
      (0-11): 12 x BertLayer(
        (attention): BertAttention(
          (self): BertSelfAttention(
            (query): Linear(in_features=768, out_features=768, bias=True)
            (key): Linear(in_features=768, out_features=768, bias=True)
            (value): Linear(in_features=768, out_features=768, bias=True)
            (dropout): Dropout(p=0.1, inplace=False)
          )
          (output): BertSelfOutput(
            (dense): Linear(in_features=768, out_features=768, bias=True)
            (LayerNorm): LayerNorm((768,), eps=1e-12, elementwise_affine=True)
            (dropout): Dropout(p=0.1, inplace=False)
          )
        )
        (intermediate): BertIntermediate(
          (dense): Linear(in_features=768, out_features=3072, bias=True)
          (intermediate_act_fn): GELUActivation()
        )
        (output): BertOutput(
          (dense): Linear(in_features=3072, out_features=768, bias=True)
          (LayerNorm): LayerNorm((768,), eps=1e-12, elementwise_affine=True)
          (dropout): Dropout(p=0.1, inplace=False)
        )
      )
    )
  )
)   
\end{lstlisting}
}

Consider the case where only two tokens are relevant for the masked token, e.g. the masked token is either ``buy'' or ``sell''.
That means, the probability distribution is only over these two tokens. 
In such case, the ratio between the probability of the two tokens is given by:
\begin{align}
    \frac{p_1}{p_2} = \frac{\exp(l_1)}{\exp(l_2)} = \exp(l_1 - l_2) = \exp(\mathbf{p} \cdot (\mathbf{x}_1 - \mathbf{x}_2) + (b_1 - b_2)).
\end{align}
Write $\mathbf{x}_1 - \mathbf{x}_2$ as $\Delta \mathbf{x}$ and $b_1 - b_2$ as $\Delta b$, then the log ratio between the probability of the two tokens is given by:
\begin{align}
    \log \frac{p_1}{p_2} = \mathbf{p} \cdot \Delta \mathbf{x} + \Delta b
\end{align}

Here, the output vector $\mathbf{p}$ and the feedforward layer $FF$ are out of our control, but we can control which two tokens are considered relevant for the masked token.
In geometric terms, every pair of tokens defines a hyperplane in the embedding space, and the log ratio between the probability of the two tokens is given by the distance between the hyperplane and the output vector $\mathbf{p}$.
The hyperplane is perpendicular to the vector $\Delta \mathbf{x}$, and the signed distance between the hyperplane and the origin is given by $\Delta b/||\Delta \mathbf{x}||$.
Therefore, the log ratio between the probabilities $\log \frac{p_1}{p_2}$ is the distance between the output vector $\mathbf{p}$ and the hyperplane defined by the two tokens.

% draw a picture here using tikz
\begin{figure}[h] 
  \centering
\begin{tikzpicture}[scale=1]

    % Set variables
    \def\xmin{-1}
    \def\xmax{3}
    \def\ymin{-1}
    \def\ymax{3}
    \def\kx{1}
    \def\ky{2}
    \def\b{2}

    % Set up the Cartesian coordinate system
    \draw[->] (\xmin,0) -- (\xmax,0) node[right] {};
    \draw[->] (0,\ymin) -- (0,\ymax) node[above] {};
    
    % Draw grid lines
    % \draw[gray!30, step=1] (\xmin,\ymin) grid (\xmax,\ymax);

    % Draw the line (hyperplane)
    \draw[thick] (\xmin,{-\kx/\ky*\xmin + \b/\ky}) -- (\xmax,{-\kx/\ky*\xmax + \b/\ky}) node[right] {$0 = \mathbf{p} \cdot \Delta \mathbf{x} + \Delta b$};

    % Draw the vector \vec{k}
    % \draw[->,red,thick] (0,0) -- (\kx,\ky) node[anchor=south east] {$\vec{k}$};

    % Calculate the distance d from the origin to the line
    % The point on the line closest to the origin is (d * k_x / ||k||, d * k_y / ||k||)
    \pgfmathsetmacro{\normk}{sqrt(\kx*\kx + \ky*\ky)}
    \pgfmathsetmacro{\d}{abs(\b) / \normk}
    \pgfmathsetmacro{\dx}{\d * \kx / \normk}
    \pgfmathsetmacro{\dy}{\d * \ky / \normk}
    \draw[->,red,thick] (0,0) -- (\dx,\dy) node[anchor=south] {$\frac{\Delta b}{\Vert \Delta x \Vert} $};
\end{tikzpicture}
\end{figure}

\section{BERT and contextuality}
The PR like schema defines a PR-like model, where the parameters $\epsilon_i$ are determined specific words chosen.
BERT provides the probabilities $p_{i, i \oplus 1}$, which are filled an empirical table:
\begin{table}[h]
  \centering
  \begin{tabular}{r|ccccc}
  & $(0, 0)$ & $(0, 1)$ & $(1, 0)$ & $(1, 1)$  \\ \hline
  $(x_1, x_2)$ & $p_{1,2}$ & $0$ & $0$ & $1-p_{1,2}$ \\
  $(x_2, x_3)$ & $p_{2,3}$ & $0$ & $0$ & $1-p_{2,3}$ \\
  $(x_3, x_4)$ & $p_{3,4}$ & $0$ & $0$ & $1-p_{3,4}$ \\
  $(x_4, x_1)$ & $0$ & $p_{4,1}$ & $1-p_{4,1}$ & $0$ \\
  \end{tabular}
\end{table}
Thus the epsilon parameters are given by:
\begin{align}
    \epsilon_{i, i \oplus 1} = 2 p_{i, i \oplus 1} - 1.
\end{align}
The log ratio between the probabilities of the two tokens can be written in terms of the epsilon parameters as follows:
\begin{align}
  \log \frac{1+\epsilon_{i, i \oplus 1}}{1-\epsilon_{i, i \oplus 1}} = \mathbf{p_{i, i \oplus 1}} \cdot \Delta \mathbf{x} + \Delta b
\end{align}
where $\mathbf{p}_{i, i \oplus 1}$ is the contextualised output vector of the masked token for the context $(x_i, x_{i \oplus 1})$.
Rearrange the above to get
\begin{align}
    \epsilon_{i, i \oplus 1} = \tanh\left(\frac{1}{2}(\mathbf{p_{i, i \oplus 1}} \cdot \Delta \mathbf{x} + \Delta b)\right).
\end{align}
where $\tanh(x) = \frac{e^x - e^{-x}}{e^x + e^{-x}}$ is the hyperbolic tangent function.
Thus the signalling fraction can be seen as the maximum absolute deviation from the hyperplane defined by the two nouns in the example of the schema.
Unfortunately, the geometric interpretation of the Direct influence is not as clear.

\section{A break down of BERT}
In this section we try to break down the BERT model into its components, and see how each component contributes to the contextualisation of the output vectors.

{
\footnotesize
\begin{lstlisting}
BertForMaskedLM(
  (bert): BertModel(
    (embeddings): BertEmbeddings(
      ...
    )
    (encoder): BertEncoder(
      ...
    )
  )
  (cls): BertOnlyMLMHead(
   ...
  )
)
\end{lstlisting}    
}

We can see that the BERT model is composed of three components: the embedding layer, the encoder, and the prediction head.

\subsection{Embedding layer}
% show the embedding layer
{
\footnotesize
\begin{lstlisting}
BertEmbeddings(
  (word_embeddings): Embedding(30522, 768, padding_idx=0)
  (position_embeddings): Embedding(512, 768)
  (token_type_embeddings): Embedding(2, 768)
  (LayerNorm): LayerNorm((768,), eps=1e-12, elementwise_affine=True)
  (dropout): Dropout(p=0.1, inplace=False)
)
\end{lstlisting}    
}
The embedding layer simply converts a sequence of token ids into a sequence of embedding vectors, according to a trainable lookup table.
Positional embeddings are added to the embedding vectors to indicate the position of each token in the sequence.
A token type embedding is also added to each token, to indicate whether the token belongs to the first sentence or the second sentence.
This is followed by a normalisation which ensures that the components of the embedding vectors have zero mean and unit variance.
Finally, a dropout layer is applied to the embedding vectors to prevent overfitting during training.

\subsection{Encoder}
% show the encoder
{
\footnotesize
\begin{lstlisting}
BertEncoder(
  (layer): ModuleList(
    (0-11): 12 x BertLayer(
      ...
    )
  )
)
\end{lstlisting}    
}

The BERT encoder is a stack of 12 identical layers.

% show one layer
{
\footnotesize
\begin{lstlisting}
BertLayer(
  (attention): BertAttention(
    (self): BertSelfAttention(
      (query): Linear(in_features=768, out_features=768, bias=True)
      (key): Linear(in_features=768, out_features=768, bias=True)
      (value): Linear(in_features=768, out_features=768, bias=True)
      (dropout): Dropout(p=0.1, inplace=False)
    )
    (output): BertSelfOutput(
      (dense): Linear(in_features=768, out_features=768, bias=True)
      (LayerNorm): LayerNorm((768,), eps=1e-12, elementwise_affine=True)
      (dropout): Dropout(p=0.1, inplace=False)
    )
  )
  (intermediate): BertIntermediate(
    (dense): Linear(in_features=768, out_features=3072, bias=True)
    (intermediate_act_fn): GELUActivation()
  )
  (output): BertOutput(
    (dense): Linear(in_features=3072, out_features=768, bias=True)
    (LayerNorm): LayerNorm((768,), eps=1e-12, elementwise_affine=True)
    (dropout): Dropout(p=0.1, inplace=False)
  )
)
\end{lstlisting}    
}
The last two modules in each layer are the intermediate layer and the output layer, which are just two feedforward layers with a GELU activation function in between, following by a layer normalisation and a dropout layer.
The main component is the BertAttention module, which mixes information from different positions in the sequence.
It does so by first computing three vectors for each token: a query vector, a key vector, and a value vector. These vectors have the same dimension as the embedding vectors.
The query vector is used to compute the attention weights between the tokens in the sequence, by taking the dot product between the query vector and the key vector of each token.
The attention weights are then used as the weights in a weighted sum of the value vectors, to produce the output vector for each token.
In multi-head attention, the labour of producing the output vector is split between multiple smaller attention modules, each of which is called a head.
The three vectors are still computed from all the components of the embedding vectors, but their dimension is as just as large as the part of the output vector that is produced by the head.
For example, in bert-base-uncased, the embedding size is 768, and the number of heads is 12, so each head produces an output vector of size 64, and the dimension of the query, key, and value vectors is 64.
These output vectors from each head are then concatenated to produce the final output vector of size 768.
At this point, each token position has an contextualised embedding vector that is a mixture of the embedding vectors of all the tokens in the sequence.

The BertSelfOutput is just another feedforward layer with a layer normalisation and a dropout layer. 

\subsection{Prediction head}
% show the prediction head
{
\footnotesize
\begin{lstlisting}
BertOnlyMLMHead(
  (predictions): BertLMPredictionHead(
    (transform): BertPredictionHeadTransform(
      (dense): Linear(in_features=768, out_features=768, bias=True)
      (transform_act_fn): GELUActivation()
      (LayerNorm): LayerNorm((768,), eps=1e-12, elementwise_affine=True)
    )
    (decoder): Linear(in_features=768, out_features=30522, bias=True)
  )
)
\end{lstlisting}    
}

The transform module is just another feedforward layer with a GELU activation function in between, following by a layer normalisation.
The decoder is a linear layer that converts the output vector into a vector of logits, one for each token in the vocabulary.
The weights used in this linear layer are the embedding vectors of the tokens in the vocabulary. Thus the logits are computed by taking the dot product between the output vector and the embedding vectors of the tokens in the vocabulary, followed by a scalar bias term (which is different for each token in the vocabulary).

\subsection{notations}
We define the input embeddings of a sequence as $(\mathbf{x}_0, \mathbf{x}_1, \cdots, \mathbf{x}_n, \mathbf{x}_{n+1})$,
where $\mathbf{x}_0$ is the embedding vector of the special token [CLS], the $\mathbf{x}_i$ are the embedding vectors of the tokens in the sequence, and $\mathbf{x}_{n+1}$ is the embedding vector of the special token [SEP].

We denote the output embeddings of the encoder as $(\mathbf{y}_0, \mathbf{y}_1, \cdots, \mathbf{y}_n, \mathbf{y}_{n+1})$.
We denote the output embeddings of the prediction head as $(\mathbf{p}_0, \mathbf{p}_1, \cdots, \mathbf{p}_n, \mathbf{p}_{n+1})$.

\begin{figure}[h]
    \centering
\input{figures/bert_flow.tex}
\caption{A flow chart of the BERT model illustrating how the embedding vectors are transformed into the output vectors.}
\end{figure}
